# Supplementary material for: RP-DNN: A Tweet level propagation context based deep neural networks for early rumor detection in Social Media
Source: arXiv:2002.12683 source file (2020-03-02)
Supplement: Supplementary file 1 [file appendices.tex]

\section{Appendices}\label{appendices}

Table \ref{tab:appendix_globalnorm} presents the global means and standard deviation computed from whole training set and used to normalise feature representations of context metadata.

\begin{table*}[t]
{\footnotesize\begin{tabular}{
            p{\dimexpr 0.12 \linewidth-2.4\tabcolsep}
				p{\dimexpr 0.25 \linewidth-2.8\tabcolsep}
				p{\dimexpr 0.15 \linewidth-2.6\tabcolsep}
				p{\dimexpr 0.15 \linewidth-2.6\tabcolsep}
				p{\dimexpr 0.15 \linewidth-3.0\tabcolsep}
				p{\dimexpr 0.15 \linewidth-3.0\tabcolsep}}
\multirow{1}{*}{\bf } & \bf NFs & \bf global mean & \bf global std. & \bf global max & \bf global min \\ \hline
\multirow{4}{*}{user features} & \# of posts & 53687.5965 & 127457.9930 & 4420429 & 1 \\	
    & listed count & 102.4828 & 1228.3984 & 199211 & 0 \\
    & followers & 7174.8032 & 233721.4625 & 42822106 & 0 \\
    & followings & 1679.2319 & 8920.4870 & 1602789 & 0 \\
    & follow ratio & 163.1336 & 31374.2225 & 9918751.75 & 0\\ 
    & follow ratio (v2) & 0.4722 & 0.2282 & 1 & 0 \\ 
    & \# of user favourites & 18493.6203 & 49741.6807 & 2419251 & 0 \\
    & account age & 1197.2359 & 686.5547 & 3611 & 1 \\
    & is verified & 0.0269 & 0.1618 & 1 & 0 \\
    & engagement scr & 82.5727 & 534.0954 & 164474.5 & 0.0005 \\
    & following rate & 3.7328 & 32.6771 & 6207.4 & 0 \\
    & favourites scr & 38.3545 & 407.0863 & 85537 & 0 \\ 
    & is GEO enabled & 0.5282 & 0.4992 & 1 & 0 \\ 
    & description length & 11.7235 & 8.7322 & 64 & 0 \\
    & user profile name length & 11.6878 & 5.5836 & 50 & 0 \\
    & is source user & 0.0098 & 0.0987 & 1 & 0 \\ \hline
\multirow{3}{*}{tweet features} & \# of retweets & 263.1094 & 1040.1257 & 77459 & 0 \\
    & \# of favorites & 0.3600 & 36.3189 & 22836 & 0 \\
    & has question & 0.0579 & 0.2336 & 1 & 0 \\
    & is duplicated & 0.0011 & 0.0324 & 1 & 0 \\
    & has image & 0.8762 & 0.3294 & 1 & 0 \\
    & has URL & 0.3083 & 0.4618 & 1 & 0 \\
    & \# of URL & 0.31187853 & 0.4712 & 5 & 0 \\
    & has native media & 0.1679 & 0.3738 & 1 & 0 \\
    & context content length & 15.8925 & 5.5011 & 47 & 0 \\
    & response time decay (mins.) & 1664.1876 & 42754.3823 & 3152616.7667 & 0 \\
    % & context type  & 0.2117 & 0.4085 & 1 & 0 \\
    & has user profile desc  & 0.8529 & 0.3542 & 1 & 0 \\\hline
\end{tabular}}{\caption{Statistics of global Mean-variance in whole training set}
      \label{tab:appendix_globalnorm}}
\end{table*}
